# Supplementary material for: A theory of cut-restriction: first steps
Source: arXiv:2203.01600 source file (2022-03-03)
Supplement: Supplementary file 1 [file appendix.tex]

\section*{Appendix}

We provide a full proof for Lemma~\ref{lem:adminv}.

The induction is on the height $h$ of a proof deriving the respective premise of that rule, where one assumes that locally analytic hp-admissibility/invertibility has been shown for \textit{all} rules mentioned in the Lemma whenever their premise admits a proof of height $<h$.

Consider first the case that $h=1$, so that the premise is an initial sequent of $\BiInt$. Clearly all initial sequents are closed under adding formulas or removing duplicate formulas, and therefore we have the admissibility of the contraction and weakening rules.

Now for the logical rules, let us consider any formula $C$ occuring in an initial sequent. If $C$ is either (a) a conjunction $A\land B$ or (b) a disjunction $A\lor B$ or (c) the constant $\top$ appearing in the antecedent or (d) the constant $\bot$ appearing in the succedent, then $C$ must be in the weakening context (Definition~\cite{def:weakcont}) of the initial sequent. Therefore replacing $C$ by any of $A/B/\{A,B\}/\emptyset$ results again in an initial sequent. From this the invertibility of the logical rules follows.

Let us move to the case $h>1$. For each of the rules in question, we make a case distinction on the last rule $r$ applied in the derivation of its premise. 

\begin{itemize}
    \item $\top_L$:
\begin{itemize}
    \item $r=\cut$ with cut formula $C\neq \top$:
\[
\infer[\cut]{\Gamma,\top\Sa\Delta}
    {
    \Gamma,\top\Sa C,\Delta
    &
    \Gamma,\top,C\Sa\Delta
    }
\quad
\overset{C\neq \top}{\leadsto}
\quad
\infer[cut]{\Gamma\Sa\Delta}
    {
    \infer[IH]{\Gamma\Sa C,\Delta}
        {
        \Gamma,\top\Sa C,\Delta
        }
    &
     \infer[IH]{\Gamma,C\Sa \Delta}
        {
        \Gamma,\top,C\Sa \Delta
        }
    }
\]

Note that the cut on $C$ could cease to be analytic only if $C=\top$. It follows from this and the induction hypothesis that the transformed proof has no more non-analytic cuts.

\item $r=\cut$ with cut formula $C=\top$:
\[
\infer[\cut]{\Gamma,\top\Sa\Delta}
    {
    \Gamma,\top\Sa C,\Delta
    &
    \Gamma,\top,C\Sa\Delta
    }
\quad
\overset{C=\top}{\leadsto}
\quad
\infer[IH]{\Gamma\Sa\Delta}
    {
    \infer[IH]{\Gamma,\top\Sa\Delta}
        {
        \Gamma,\top,C\Sa\Delta
        }
    }
\]
Here we first apply the IH to contract $\top,C$ into $\top$. As height is preserved, we can then apply the IH again to remove $\bot$.
\end{itemize}
\end{itemize}
\item $\land_L$:
\begin{itemize}
    \item $r=\cut$ with cut formula $C\neq A\land B$:
    \[
    \infer[\cut]{\Gamma,A\land B\Sa\Delta}
        {
        \Gamma,A\land B\Sa C,\Delta
        &
        \Gamma,A\land B,C\Sa\Delta
        }
    \quad
    \leadsto
    \quad
    \infer[cut]{\Gamma,A,B\Sa\Delta}
        {
        \infer[IH]{\Gamma,A,B\Sa C,\Delta}
            {
            {\Gamma,A\land B\Sa C,\Delta}
            }
        &
        \infer[IH]{\Gamma,A,B,C\Sa \Delta}
            {
            {\Gamma,A\land B,C\Sa \Delta}
            }
        }
    \]
    Note that if the cut on $C$ was analytic before the transformation, then it remains so afterwards. However by appeal to IH we may have introduced non-analytic cuts on subformulas of $A$ and $B$.
    \item $r=\cut$ with cut formula $C=A\land B$:
    \[
    \infer[\cut]{\Gamma,A\land B\Sa\Delta}
        {
        \Gamma,A\land B\Sa C,\Delta
        &
        \Gamma,A\land B,C\Sa\Delta
        }
    \quad
    \leadsto
    \quad
    \infer[IH]{\Gamma,A\Sa\Delta}
        {
        \infer[IH]{\Gamma,A\land B\Sa\Delta}
            {
            \Gamma,A\land B,C\Sa\Delta
            }
        }
    \]
\end{itemize}

\item $\contr_L$
\end{itemize}
